# Supplementary material for: Magnetic Field Dependent Microwave Losses in Superconducting Niobium Microstrip Resonators
Source: arXiv:1802.05183 source file (2018-06-26)
Supplement: Supplementary file 1 [file supp.pdf]

# Supplementary Materials

## S1 Time-dependent Ginzburg–Landau Equations

The time-dependent Ginzburg–Landau (GL) equations are given by (in SI units)[65,100,101]

$$-\frac{\hbar^2}{2m_sD}\left(\frac{\partial}{\partial t}+\frac{ie_s}{\hbar}\phi\right)\psi=\alpha\psi+\beta|\psi|^2\psi+\frac{1}{2m_s}\left(\frac{\hbar}{i}\nabla-e_s\vec{A}\right)^2\psi, \tag{S1}$$

$$\frac{1}{\mu_0}\nabla\times\nabla\times\vec{A}=\frac{e_s\hbar}{2m_si}\left(\psi^*\nabla\psi-\psi\nabla\psi^*\right)-\frac{e_s^2}{m_s}|\psi|^2\vec{A}+\sigma_n\left(-\frac{\partial\vec{A}}{\partial t}-\nabla\phi\right), \tag{S2}$$

where $\psi=\psi(x,y,z,t)$ is the complex order parameter; $\alpha$ and $\beta$ are phenomenological parameters; $D$ is the phenomenological diffusion coefficient; $e_s$ and $m_s$ are the charge and the mass of the superconducting electron, respectively; $\vec{A}$ is the magnetic vector potential; $\phi$ is the electric potential; and $\sigma_n$ is the inverse of the residual resistivity. The applied magnetic field $\vec{H}_a$ is assumed uniform, $\nabla\times\vec{H}_a=0$.

Boundary conditions at the surface of a superconducting sample are given by

$$\nabla\times\vec{A}=\mu_0\vec{H}_a,\quad \vec{J}_s\cdot\vec{n}=0,\quad \sigma_n\vec{E}\cdot\vec{n}=0, \tag{S3}$$

where $J_s$ is the supercurrent density. The last two conditions ensure that no current passes through the surface. These conditions can also be written as

$$\left(\frac{\hbar}{i}\nabla\psi-e_s\vec{A}\psi\right)\cdot\vec{n}=0,\quad \left(\frac{\partial\vec{A}}{\partial t}+\nabla\phi\right)\cdot\vec{n}=0. \tag{S4}$$

We transform the GL equations into dimensionless quantities by measuring length in units of the penetration depth $\lambda$; time in units of the characteristic relaxation time $\tau\equiv\xi^2/D$, where $\xi$ is the GL coherence length; fields in units of $\sqrt{2}H_c$, where $H_c$ is the thermodynamic critical field; and order parameter in units of $\psi_0\equiv\sqrt{|\alpha|/\beta}$. Then, Eqs. (S1) and (S2) become[101]

$$\left(\frac{\partial}{\partial t}+i\kappa\phi\right)\psi=-\left(\frac{i}{\kappa}\nabla+\vec{A}\right)^2\psi+\psi-|\psi|^2\psi, \tag{S5}$$

$$\sigma_n\left(\frac{\partial\vec{A}}{\partial t}+\nabla\phi\right)=\frac{1}{2i\kappa}\left(\psi^*\nabla\psi-\psi\nabla\psi^*\right)-|\psi|^2\vec{A}-\nabla\times\nabla\times\vec{A}, \tag{S6}$$

where $\kappa\equiv\lambda/\xi$ is the GL parameter.

The time-dependent GL equations are invariant under the gauge transformation with a function $\chi(x,y,z,t)$:

$$\tilde{\psi}=\psi e^{i\kappa\chi},\quad \tilde{\vec{A}}=\vec{A}+\nabla\chi,\quad \tilde{\phi}=\phi-\frac{\partial\chi}{\partial t}.$$

For convenience, we choose the zero-electric potential gauge, $\tilde{\phi}=0$. Dropping tildes, Eqs. (S5) and (S6) are written as

$$\frac{\partial\psi}{\partial t}=-\left(\frac{i}{\kappa}\nabla+\vec{A}\right)^2\psi+\psi-|\psi|^2\psi, \tag{S7}$$

$$\sigma_n\frac{\partial\vec{A}}{\partial t}=\frac{1}{2i\kappa}\left(\psi^*\nabla\psi-\psi\nabla\psi^*\right)-|\psi|^2\vec{A}-\nabla\times\nabla\times\vec{A}. \tag{S8}$$

The equations for the boundary conditions, Eqs. (S3) and (S4), become

$$\nabla \times \vec{A} - \mu_0 \vec{H}_\mathrm{a} = 0, \quad \nabla\psi \cdot \vec{n} = 0, \quad \vec{A} \cdot \vec{n} = 0. \tag{S9}$$

Hence the steady-state solutions of Eqs. (S7) and (S8) are determined by $\vec{A}$, $d/\lambda$, and $\kappa$, where $d$ is the film thickness.

To solve Eqs. (S7)–(S9), COMSOL Multiphysics 5.1 was used. We closely followed the implementation introduced in Ref. 102. The general form of partial differential equations in COMSOL Multiphysics is

$$\mathbf{e}_a \frac{\partial^2 \mathbf{u}}{\partial t^2} + \mathbf{d}_a \frac{\partial \mathbf{u}}{\partial t} + \nabla \cdot \mathbf{\Gamma} = \mathbf{f}. \tag{S10}$$

All geometries were assumed to be two-dimensional systems on the $xy$ plane. $\vec{H}_\mathrm{a}$ is assumed to be along the $z$ direction. In this case, $\mathbf{u} = (u_1, u_2, u_3, u_4, u_5)^\mathrm{T}$, where T is the transpose. The variables are given by $u_1(x, y, t) = \mathrm{Re}(\psi(x, y, t))$, $u_2(x, y, t) = \mathrm{Im}(\psi(x, y, t))$, $u_3(x, y, t) = A_x(x, y, t)$, and $u_4(x, y, t) = A_y(x, y, t)$, respectively. To satisfy the boundary conditions, we need five differential equations. Thus, an auxiliary variable $u_5$ is introduced, which is always zero.

In Eq. (S10), $\mathbf{e}_a$ is a zero matrix. Others can be written as

$$\mathbf{d}_a = \begin{bmatrix} 1 & 0 & 0 & 0 & 0 \\ 0 & 1 & 0 & 0 & 0 \\ 0 & 0 & \sigma_\mathrm{n} & 0 & 0 \\ 0 & 0 & 0 & \sigma_\mathrm{n} & 0 \\ 0 & 0 & 0 & 0 & 0 \end{bmatrix}, \quad \mathbf{\Gamma} = \begin{bmatrix} [-\partial_x u_1/\kappa^2, -\partial_y u_1/\kappa^2]^\mathrm{T} \\ [-\partial_x u_2/\kappa^2, -\partial_y u_2/\kappa^2]^\mathrm{T} \\ [0, \partial_x u_4 - \partial_y u_3 - \mu_0 H_\mathrm{a}]^\mathrm{T} \\ [-\partial_x u_4 + \partial_y u_3 + \mu_0 H_\mathrm{a}, 0]^\mathrm{T} \\ [u_3, u_4]^\mathrm{T} \end{bmatrix},$$

$$\mathbf{f} = \begin{bmatrix} (\partial_x u_3 + \partial_y u_4) u_2/\kappa + 2(u_3 \partial_x u_2 + u_4 \partial_y u_2)/\kappa - (u_3^2 + u_4^2) u_1 + u_1 - (u_1^2 + u_2^2) u_1 \\ -(\partial_x u_3 + \partial_y u_4) u_1/\kappa - 2(u_3 \partial_x u_1 + u_4 \partial_y u_1)/\kappa - (u_3^2 + u_4^2) u_2 + u_2 - (u_1^2 + u_2^2) u_2 \\ (u_1 \partial_x u_2 - u_2 \partial_x u_1)/\kappa - (u_1^2 + u_2^2) u_3 \\ (u_1 \partial_y u_2 - u_2 \partial_y u_1)/\kappa - (u_1^2 + u_2^2) u_4 \\ \partial_x u_3 + \partial_y u_4 + u_5 \end{bmatrix}.$$

The boundary conditions were implemented using "zero flux" $-\vec{n} \cdot \mathbf{\Gamma} = \mathbf{G}$, where $\mathbf{G} = [0, 0, 0, 0, 0]^\mathrm{T}$.

Setting proper initial values allows us to imitate cooling procedures, and consequently, to obtain the Bean–Livingston surface barrier naturally from the GL equations. All simulations shown in the main text were obtained with the initial condition for the zero-field cooling procedure: we set the initial condition as $u_1 = 1$, $u_2 = u_3 = u_4 = u_5 = 0$.

For Fig. 6, $\kappa$ is 10 and the width of the slap along the $x$ axis is $10\lambda$. We apply a periodic boundary condition on the $z$ axis, and the distance between the two boundaries is $2\lambda$.

The mesh size is $\lambda_0/20$ for Fig. 4 and $\lambda_0/100$ for Fig. 6.

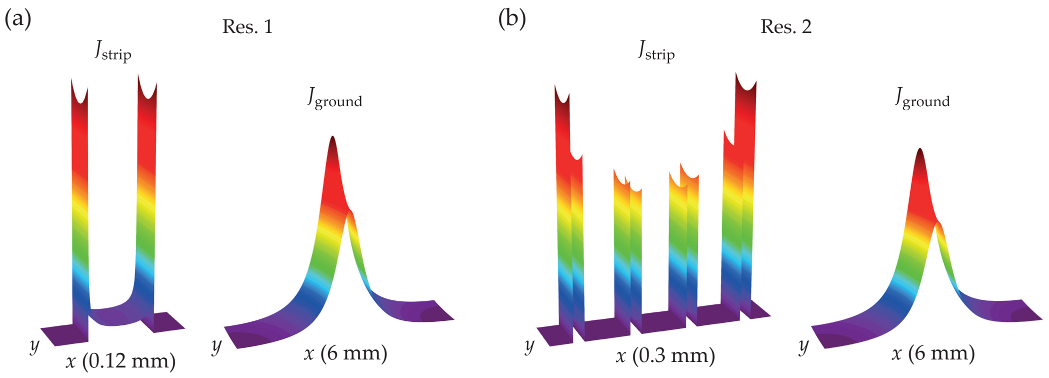


Figure S1: Numerically calculated microwave current density distribution of Res. 1 and 2. We assume the strips and the ground plane have the same penetration depth of $\lambda = 52$ nm. Both $J_{\text{strip}}$ and $J_{\text{ground}}$ are on an arbitrary scale; in practice, $J_{\text{ground}}$ is orders of magnitude lower than $J_{\text{strip}}$. The numbers in parenthesis indicate the range of the plot.

# S2 Microwave Current Density Distribution and Stored Electromagnetic Energy

To calculate the microwave current density distribution and the electromagnetic energy of our resonator, the London equations needed to be incorporated into Maxwell's equations. This was achieved by parameterizing the penetration depth via the complex conductivity (Eq. (8)).[103] As our resonators are straight strips, we did not need to consider the axis along the strip ($z$ axis). By considering only the $xy$ plane, we were able to simulate the entire cross section of the resonator packages.

The calculations were carried out using COMSOL Multiphysics 5.1 (AC/DC module). For the strips and the ground plane, the mesh sizes varied from $d/200$ to 0.5 mm. We confirmed our method by calculating several analytically solvable geometries[104] and the geometry of Ref. 103.

The microwave current density distribution of the strips $J_{\text{strip}}$ and the ground plane $J_{\text{ground}}$ of Res. 1 and 2 are shown in Fig. S1. The calculations show that the ratio of $J_z^2$ between the center of the strip, and the edges are about 400:1 and 100:1 for Res. 1 and 2 ($\lambda = 52$ nm), about 10:1 for Res. 3 ($\lambda = 162$), and about 800:1 for Res. 4 ($\lambda = 43$).

For all calculations, the value of $\lambda$ for the strip and the ground plane was kept the same. This is a reasonable assumption, because the penetration depth dependence of integrated $J^2_{\text{ground}}$ is weak: $J^2_{\text{ground}}$ changes only about 4% from $\lambda = 50$ nm to 1000 nm.

# S3 Loss Parameters for Quasiparticle Generation

In this section, we explain how to extract the loss parameters associated with quasiparticle generation from Fig. 4.

1. Calculate $n_{\mathrm{s}}$ as a function of $H_{\|}$ by solving the GL equations as described in Sec. S1; $\lambda_0$ and $\kappa$ are required for this step.
2. Once we have $n_{\mathrm{s}}(H_{\|})$, $\lambda(H_{\|})$ is obtained by

$$\left(\frac{\lambda_0}{\lambda}\right)^2 = \frac{n_{\mathrm{s}}(H_{\|})}{n_{\mathrm{s}}(0)}. \tag{S11}$$

   Equation (S11) is derived from Eq. (8). Once $\lambda$ is known, $J_{\mathrm{strip}}$ and $L_{\mathrm{mag}}$ are calculated as described in Sec. S2.
3. $f^{-2}$ is reconstructed theoretically using Eqs. (4)–(8); $H_{\mathrm{c}}$ is required for this step.
4. Repeat Steps 1–3 until theoretical $f^{-2}$ is sufficiently close to the experimental results. Then, $\lambda_0$, $\kappa$, and $H_{\mathrm{c}}$ are determined.
5. Using $n_{\mathrm{s}}(H_{\|})$ from the $f^{-2}$ data, $Q_{0,\mathrm{fit}}$, $\rho_{\mathrm{n,fit}}$, and $\beta$ are determined using a similar procedure with $Q^{-1}$. In order to calculate $Q^{-1}$, the following expression for $\sigma_{\mathrm{tf},1}$ was used, which is based on Eq. (10):

$$\sigma_{\mathrm{tf},1} = \left[1 - \frac{n_{\mathrm{s}}(H_{\|})}{n_{\mathrm{s}}(0)}\right]^{\beta} \frac{1}{\rho_{\mathrm{n,fit}}}.$$

We remark that $\sigma_{\mathrm{tf},1} \ll \sigma_{\mathrm{tf},2}$ for most of the magnetic field range and $\rho_{\mathrm{tf},2} = \sigma_{\mathrm{tf},2}/(\sigma_{\mathrm{tf},1}^2 + \sigma_{\mathrm{tf},2}^2)$. As a result, $\rho_{\mathrm{n,fit}}$ and $\beta$ contribute to $f^{-2}$ very little, and one can fit $f^{-2}$ first. Note that a log-linear plot should be used, as shown in Fig. 4(a). The fitting for Fig. 4(b) was also done using the $Q^{-1}$ vs. $H_{\|}$ plot in a log-linear scale. The reason is that, although the changes to $f^{-2}$ and $Q^{-1}$ at low fields are small, they are crucial to obtain accurate loss parameters.

A crude description of the role of each fitting parameter is as follows: The curvature of $n_{\mathrm{s}}$ below the vortex penetration field is determined mostly by $\lambda_0$, above the vortex penetration field the curvature is determined by $\kappa$. $H_{\mathrm{c}}$ scales $n_{\mathrm{s}}$ along the $H_{\|}$-axis. For $Q^{-1}$, $\beta$ determines the curvature, $A_{\mathrm{n}}$ adjusts the scale along the $Q^{-1}$ axis, and $Q_{0,\mathrm{fit}}$ is the intercept on the $Q$ axis in Fig. 4(b).

During the calculations, the ground plane's contribution was assumed negligible, hence $\lambda_0$ in Eq. (S11) is the zero-field penetration depth of the strips. The reason is that ground plane's contribution to the microwave current density is just a few percent. If the ground plane becomes normal prior to the strips, then its contribution might be comparable to that of the strips. To avoid such a complication, we kept the film thickness of the ground plane the same as that of the strips. As the ground plane is dirtier than the strips (see Table I and Sec. S5), its upper critical field is expected to be higher.

# S4 Loss Parameters for Vortex Motion

In this section, we explain how to determine the loss parameters associated with vortex motion.

For the data taken after the heat-pulsing procedure, the procedure is more straightforward than that described in Sec. S3 because a homogeneous vortex distribution results in the complex resistivity proportional to $H_\perp$ (Eq. (13)).

Using equations Eqs.(1)–(6), (12), and (13), we find:

$$\frac{f^{-2}-f_{\mathrm{bg}}^{-2}}{f_{\mathrm{bg}}^{-2}} = \frac{L-L_{\mathrm{bg}}}{L_{\mathrm{bg}}} \approx \frac{\Phi_0 B_\perp}{\eta}\frac{\omega/\omega_{\mathrm{eff}}(1-\epsilon)}{1+(\omega/\omega_{\mathrm{eff}})^2}\frac{1}{\omega}\frac{\int_{\mathrm{sc}}|J_{\mathrm{mw}}(x,y,\lambda)|^2dxdy}{\int_{\mathrm{all}}\mu_0|H_{\mathrm{mw}}(x,y,\lambda)|^2dxdy}, \tag{S12}$$

$$Q^{-1}-Q_{\mathrm{bg}}^{-1} = \frac{P_{\mathrm{diss}}}{\omega U_{\mathrm{em}}} \approx \frac{\Phi_0 B_\perp}{\eta}\frac{(\omega/\omega_{\mathrm{eff}})^2+\epsilon}{1+(\omega/\omega_{\mathrm{eff}})^2}\frac{1}{\omega}\frac{\int_{\mathrm{sc}}|J_{\mathrm{mw}}(x,y,\lambda)|^2dxdy}{\int_{\mathrm{all}}\mu_0|H_{\mathrm{mw}}(x,y,\lambda)|^2dxdy}, \tag{S13}$$

where $L_{\mathrm{bg}} \equiv L(H_\parallel = H_{\mathrm{bg}}, \theta = 0)$.

If vortex motion contributes dominantly to the complex resistivity, i.e., $[\rho_{\mathrm{tf},i}(H_\perp) - \rho_{\mathrm{tf},i}(0)] \ll \rho_{\mathrm{vm},i}$, and $\epsilon$ is negligibly small, then we can extract the $r$-parameter using Eqs. (S12) and (S13):[66]

$$r(H_\perp) \equiv \frac{\rho_{\mathrm{vm},2}(H_\perp)}{\rho_{\mathrm{vm},1}(H_\perp)} = \frac{(f^{-2}-f_{\mathrm{bg}}^{-2})/f_{\mathrm{bg}}^{-2}}{Q^{-1}-Q_{\mathrm{bg}}^{-1}} \approx \frac{\omega_{\mathrm{p}}}{\omega}. \tag{S14}$$

Using Eq. (S14), the $r$-parameter of each data point can be obtained. Once we have $r$, we can obtain $\omega_{\mathrm{p}}(= r\omega)$. For Table III, we used the average $r$ value for all HP data points using the ratio between the slopes of $(f^{-2}-f_{\mathrm{bg}}^{-2})/f_{\mathrm{bg}}^{-2}$ and $Q^{-1}-Q_{\mathrm{bg}}^{-1}$; the slopes were obtained by linear fitting. (For Res. 3, the zero-field cooling data above 14 mT were used because of the absence of the heat-pulsing data.)

Here, $\eta$ can be calculated using either Eq. (S12) or (S13); we used Eq. (S12), because the measurement accuracy of $f$ is better than that of $Q$.

$$\eta \approx \frac{\mu_0 H_\perp}{(f^{-2}-f_{\mathrm{bg}}^{-2})/f_{\mathrm{bg}}}\frac{\int_{\mathrm{sc}}|J_{\mathrm{mw}}(x,y,\lambda_{\mathrm{bg}})|^2dxdy}{\int_{\mathrm{all}}\mu_0|H_{\mathrm{mw}}(x,y,\lambda_{\mathrm{bg}})|^2dxdy}\frac{\Phi_0}{\omega}\frac{1}{r+r^{-1}}, \tag{S15}$$

where $\lambda_{\mathrm{bg}} \equiv \lambda(H_\parallel = H_{\mathrm{bg}}, \theta = 0)$. In Eq. (S15), the second fraction was estimated by numerical calculation (see Sec. S2), and remaining fractions were given by experimental results. Similar to the case of $r$, the inverse of the slope of $(f^{-2}-f_{\mathrm{bg}}^{-2})/f_{\mathrm{bg}}$ was used as the first fraction. Then, $k_{\mathrm{p}}$ is obtained using the relation $k_{\mathrm{p}} = \eta\omega_{\mathrm{p}}$[60,61,63,64].

Lastly, we argue why the vortex creep parameter $\epsilon$ is negligible for estimating $\omega_{\mathrm{p}}$, $\eta$, and $k_{\mathrm{p}}$. The $r$-parameter from a measurement gives the upper bound of the vortex creep factor $\epsilon_{\mathrm{max}}$:[63]

$$\epsilon_{\mathrm{max}}(r) = 1 + 2r^2 - 2r\sqrt{1+r^2}. \tag{S16}$$

At 4.2 K, we obtained $r = 2.3$ for Res. 1, resulting in $\epsilon_{\mathrm{max}} = 0.044$ from Eq. (S16). According to the Coffey–Clem model, $\epsilon$ is given by $\epsilon = [I_0(U_{\mathrm{p}}/2k_{\mathrm{B}}T)]^{-2}$, where $I_0$ is the modified Bessel function of the first kind, $U_{\mathrm{p}}$ is the height of the pinning potential, $k_{\mathrm{B}}$ is the Boltzmann constant, and $T$ is the temperature. Then, $\epsilon_{\mathrm{max}} = 0.044$ corresponds to the lower bound of the pinning potential $U_{\mathrm{p,min}} = 25$ K. Based on this, $\epsilon_{\mathrm{max}}$ at 100 mK is expected to be negligible. A similar conclusion holds for other resonators.

# S5 Niobium Thin Film Growth and Characterization

The films on wafers A and B were grown in the Omicron EVO-50 Sputter System. The base pressure was held in the order of $10^{-10}$ mBar. Prior to the deposition, we chemically cleaned the substrate, first in acetone and isopropanol solvents, followed by the standard clean 1 (SC1) process.[105] The substrate was next heated *in situ* to 1000 °C, while the chamber pressure was kept stable. Heat transfer into the transparent sapphire substrate was provided by a detachable molybdenum disc. Substrate cleaning is crucial to reduce surface losses.[106,107]

After substrate cleaning, thin films were sputtered at elevated temperatures.[108] First, a niobium film, used as the ground plane, was grown at 770 °C, while the molybdenum piece was used to transfer the heat to the substrate. Next, the molybdenum disc was detached and the substrate was flipped (all *in situ*) to grow the film for the strips. Post-deposition heat is known to reconstruct and change the crystalline orientation of niobium thin films.[109] Therefore, the film was grown at 550 °C at this stage, to minimize the reconstruction of the ground plane. The deposition rate and Ar pressure were maintained at about 1.7 Å/s and $2 \times 10^{-3}$ mBar, respectively, during the growth of the films on wafers A and B.

The films on wafer C were grown in the AJA ATC Orion Series Sputtering System. The base pressure was about $1 \times 10^{-8}$ mbar. The substrate was first Ar-sputter cleaned for 5 min under substrate bias at 50 W RF power, $7 \times 10^{-3}$ mbar Ar pressure, and 30 sccm of Ar flow. Next, we annealed the substrate at 700 °C for 1 h and then let it cool down for 7 h in a vacuum, which is long enough to ensure that the substrate reaches room temperature.

The annealing step was then followed by the deposition of the film for the strips. Afterwards, we flipped the wafer to grow the ground plane. For the ground plane, the substrate was only Ar-sputtered. Pre-deposition annealing was skipped to avoid heating the already existing film for the resonators. Both films on wafer C were deposited at room temperature; the deposition rate was around 0.6 Å/s, and Ar pressure was maintained at $4 \times 10^{-3}$ mbar

The thickness of each film was determined by fitting X-ray reflection intensity curves from grazing incident X-ray beams. The crystal orientation was obtained through the high-resolution X-ray diffraction pattern and the azimuthal X-ray diffraction data ($\phi$-scan). For wafers A and B, the out-plane crystalline orientation of the films for the strips is along the (111) direction (Table I). Such an orientation is previously reported as a result of growth at elevated substrate temperatures.[109,110] Depending on the substrate temperature, mixed orientations are also possible as observed in the ground plane of wafer A.[111]

The film quality was characterized by transport measurements using the van der Pauw method[112] on 4.7 mm×4.7 mm square chips diced before resonator fabrication. A criterion $0.5R_\mathrm{n}$, where $R_\mathrm{n}$ is the normal state resistance, was used to define $T_\mathrm{c}$.
